# Supplementary material for: Automated Discovery Has No Universally Superior Harness
Source: arXiv:2607.18235 source file (2026-07-20)
Supplement: Supplementary file 1 [file config_vector_battle_analysis_appendix.tex]

\begin{table*}[t]
\centering
\caption{\textbf{Complete config-vector majority-win leaderboard for maximum score.} Configurations are ranked by cross-pair majority-win probability over 100{,}000 iterations.}
\label{tab:config_vector_battle_max_all}
\small
\setlength{\tabcolsep}{4pt}
\begin{tabular}{rllr}
\hline
Rank & Family & Configuration & Win rate \\
\hline
1 & PUCT/UCT & PUCT, $C=1$ & 0.7609 \\
2 & PUCT/UCT & UCT, $C=0.1$ & 0.7371 \\
3 & Elite/exploit & $E=1$, $\epsilon{=}20\%$ & 0.7186 \\
4 & PUCT/UCT & PUCT, $C=10$ & 0.7097 \\
5 & PUCT/UCT & PUCT, $P=4$ & 0.6681 \\
6 & PUCT/UCT & PUCT, Halved $B$ & 0.6425 \\
7 & PUCT/UCT & PUCT, $P=2$ & 0.6251 \\
8 & B/N ablation & Eighth $B$ & 0.5854 \\
9 & PUCT/UCT & UCT, $P=2$ & 0.5718 \\
10 & Elite/exploit & $E=1$, $\epsilon{=}0\%$ & 0.5681 \\
11 & Elite/exploit & $E=10$, $\epsilon{=}0\%$ & 0.4941 \\
12 & B/N ablation & Halved $B$ & 0.4531 \\
13 & PUCT/UCT & UCT, $P=4$ & 0.4355 \\
14 & PUCT/UCT & UCT, $C=1$ & 0.4187 \\
15 & PUCT/UCT & PUCT, $C=0.1$ & 0.3962 \\
16 & PUCT/UCT & PUCT, Quartered $B$ & 0.3501 \\
17 & B/N ablation & Quartered $B$ & 0.3362 \\
18 & Elite/exploit & $E=1$, $\epsilon{=}30\%$ & 0.3173 \\
19 & Elite/exploit & $E=10$, $\epsilon{=}20\%$ & 0.2939 \\
20 & PUCT/UCT & UCT, Quartered $B$ & 0.2755 \\
21 & PUCT/UCT & UCT, $C=10$ & 0.2357 \\
22 & PUCT/UCT & UCT, Halved $B$ & 0.2245 \\
23 & Elite/exploit & $E=10$, $\epsilon{=}30\%$ & 0.2160 \\
24 & OpenEvolve & Generic prompt, 1 island & 0.1066 \\
25 & Elite/exploit & $E=20$, $\epsilon{=}0\%$ & 0.0469 \\
26 & Elite/exploit & $E=20$, $\epsilon{=}30\%$ & 0.0344 \\
27 & Elite/exploit & $E=20$, $\epsilon{=}20\%$ & 0.0298 \\
28 & Elite/exploit & $E=1$, $\epsilon{=}100\%$ & 0.0019 \\
29 & OpenEvolve & Regular, 4 islands & 0.0013 \\
30 & OpenEvolve & Regular, 1 island & 0.0000 \\
\hline
\end{tabular}
\end{table*}
